# Supplementary material for: On the inclusion of the diagonal Born-Oppenheimer correction in surface hopping methods
Source: arXiv:1602.06325 ancillary file (2016-04-28)
Supplement: Supplementary file 1 [file PSSH_SuppMaterial_4.pdf]

# Supplemental Materials for "On the inclusion of the diagonal Born-Oppenheimer correction in surface hopping methods"


Rami Gherib,[1,2] Liyuan Ye,[1] Ilya G. Ryabinkin,[1,2] and Artur F. Izmaylov[1,2]

[1)] *Department of Physical and Environmental Sciences, University of Toronto Scarborough, Toronto, Ontario, M1C 1A4, Canada*

[2)] *Chemical Physics Theory Group, Department of Chemistry, University of Toronto, Toronto, Ontario M5S 3H6, Canada*



(Dated: 18 February 2016)


## I. MOMENTUM READJUSTMENT IN PSSH

When a hop occurs in FSSH, from state $|\phi_i\rangle$ to $|\phi_f\rangle$ the momentum (or velocity) is readjusted in the direction of the nonadiabatic couplings and scaled to conserve total energy

$$\mathbf{P}_f = \mathbf{P}_i + \gamma(\Delta E_{if})\mathbf{d}_{12}. \tag{1}$$

The scalling factor $\gamma$ is in practise chosen to be as small as possible. It can be readily calculated from the initial momentum ($\mathbf{P}_i$) and the difference in adiabatic potential energies ($\Delta E_{if}$).[1]

In PSSH, hops occur between phase-space PESs. This complicates the momentum readjustment procedure dramatically since a change in momentum, alters the difference between phase-space potential energy surfaces ($\Delta E^{PS}$). Note that this problem is absent in SH because $\Delta E_{ij}$ is independent on momentum. Shenvi initially proposed to scale the momentum numerically along the direction of the nonadiabatic coupling.[2] However this procedure is problematic for two main reasons: 1) It is computationally costly since it requires attempting a multitude of scaling factors at each individual time-steps until finding the one that is energy preserving. 2) This procedure requires expressing the the scaled nonadiabatic coupling vector on a grid. Unless this grid is infinitely fine, most of the time the energy preserving scaling factor will be in between grid points. Reducing the size of the grid resolves the problem, but requires more iterations. As originally pointed out,[2] an alternative way of rescaling momentum in PSSH may be advantageous.

In the remainder of this section, we construct a more efficient way of calculating $\gamma$ for hops between phase-space surfaces. Let us consider a hop from the upper phase-space surface ($E_+^{PS}$) to the lower one ($E_-^{PS}$). Let $\mathbf{P}_+$ be the momentum before the hop and $\mathbf{P}_-$ be the momentum after the hop. Both are related by $\mathbf{P}_- = \mathbf{P}_+ + \gamma \cdot \mathbf{d}_{12}$ where $\gamma$ is *a priori* unknown. $E_-^{PS}$ can thus be written

$$E_-^{PS} = \frac{(\mathbf{P}_+ + \gamma\mathbf{d}_{12})^2}{2M} + \frac{1}{2}\left(\tilde{E}_i(\mathbf{R}) + \tilde{E}_j(\mathbf{R})\right) - \frac{1}{2}\sqrt{(E_i(\mathbf{R}) - E_j(\mathbf{R}))^2 + 4\left(\frac{\mathbf{d}_{12}\cdot(\mathbf{P}_+ + \gamma\mathbf{d}_{12})}{M}\right)^2}. \tag{2}$$

The following algebraic expression are obtained when considering the difference between $E_-^{PS}$ and $E_+^{PS}$ and equating it to zero

$$0 = -\left(A\gamma + B\gamma^2 + C\right)^2 + \Delta E_{ij}{}^2 + 4\left(\frac{\mathbf{d}_{12}\cdot(\mathbf{P}_+ + \gamma\mathbf{d}_{12})}{M}\right)^2. \tag{3}$$

where

$$A = -\frac{2\mathbf{d}_{12}\cdot\mathbf{P}}{M},$$
$$B = -\frac{\mathbf{d}_{12}{}^2}{M},$$
$$C = \sqrt{\Delta E_{ij}{}^2 + 4\left(\frac{\mathbf{d}_{12}\cdot\mathbf{P}}{M}\right)^2}.$$

Expanding all terms in Eq. (3) and grouping similar powers of $\gamma$, generates a fourth order polynomial. Out of the four possible roots, two satisfy the energy conservation criterion. The $\gamma$ used is required to be real and is chosen to have the smallest magnitude. If all four roots are complex or if none of the real roots satisfy the energy conservation criterion, the hop is frustrated. Note that while the previous derivation considered a hop from $|n_+\rangle^{PS}$ to $|n_-\rangle^{PS}$, the same algorithm can be used for the reversed process. The only difference is the sign of $C$ in Eq. (3).

## II. PHASE SPACE SURFACE-HOPPING: ELECTRONIC EOMS

In PSSH, the electronic wavefunction is propagated in the basis $\left\{|n_i^{PS}(\mathbf{R};\mathbf{P})\rangle\right\}$ that diagonalizes $H^{PS}$

$$H^{PS} = \begin{pmatrix} \frac{\mathbf{P}^2}{2M} + \tilde{E}_i(\mathbf{R}) & -\frac{i\mathbf{d}_{12}\cdot\mathbf{P}}{M} \\ \frac{i\mathbf{d}_{12}\cdot\mathbf{P}}{M} & \frac{\mathbf{P}^2}{2M} + \tilde{E}_j(\mathbf{R}) \end{pmatrix}. \tag{4}$$

Hops occur between phase-space PESs according to the same heuristics as FSSH. In this section, we derive the TDSE in the phase-space representation and the hopping procedure between phase-space PES by following closely Shenvi's derivation. We also introduce small modifications and extensions of his initial work.

The TDSE for a two-level system in the adiabatic representation is

$$i\dot{c}_i = \sum_j^2 \Big( H_{ij} - i\dot{\mathbf{R}} \cdot \mathbf{d}_{ij} \Big) c_j. \tag{5}$$

To rotate the wavefunction to the phase-space representation, we introduce the following unitary matrix

$$U(\mathbf{R};\mathbf{P}) = \begin{pmatrix} \cos\left(\frac{\theta}{2}\right) e^{-i\phi/2} & -\sin\left(\frac{\theta}{2}\right) e^{-i\phi/2} \\ \sin\left(\frac{\theta}{2}\right) e^{i\phi/2} & \cos\left(\frac{\theta}{2}\right) e^{i\phi/2} \end{pmatrix}, \tag{6}$$

where

$$\tan\left(\theta(\mathbf{R};\mathbf{P})\right) = \frac{2|\mathbf{d}_{21}(\mathbf{R}) \cdot \mathbf{P}|}{(E_1(\mathbf{R}) - E_2(\mathbf{R}))M},$$
$$\frac{i\mathbf{d}_{21} \cdot \mathbf{P}}{M} = \frac{|\mathbf{d}_{21} \cdot \mathbf{P}|}{M} e^{i\phi}.$$

The implementation of the PSSH algorithm requires projecting the electronic wavefunction onto the phase-space basis

$$|\psi(t)\rangle = \sum_j^2 c_j^{PS}(t)\, |n_i^{PS}(\mathbf{R};\mathbf{P})\rangle\,. \tag{7}$$

Transformation of Eq. (5) to the phase-space representation generates

$$\dot{c}_i^{PS} = \sum_j^2 \left[ -iU^\dagger H_{ij} U - U^\dagger \Big( \mathbf{d}_{ij} \cdot \dot{\mathbf{R}} \Big) U - U^\dagger \dot{U} \right] c_j^{PS} \tag{8}$$

Since the phase-space basis is parametrically dependent on $\mathbf{R}$ and $\mathbf{P}$, the application of the chain rule makes $\dot{U}(\mathbf{R};\mathbf{P})$

$$\dot{U}(\mathbf{R};\mathbf{P}) = \sum_{ij}^2 \tilde{\mathbf{d}}_{ij} \dot{\mathbf{R}} + \tilde{\mathbf{e}}_{ij} \dot{\mathbf{P}} \tag{9}$$

where

$$\tilde{\mathbf{d}}_{ij} = \frac{\partial U_{ij}}{\partial \mathbf{R}} \qquad \tilde{\mathbf{e}}_{ij} = \frac{\partial U_{ij}}{\partial \mathbf{P}}$$

The elements $\tilde{d}_{ij}$ and $\tilde{e}_{ij}$ can also be expressed

$$\tilde{\mathbf{d}}_{ij} = \frac{\langle n_-^{PS} | \nabla_{\mathbf{R}} H^{PS} | n_+^{PS} \rangle}{E_+^{PS} - E_-^{PS}}, \tag{10}$$

$$\tilde{\mathbf{e}}_{ij} = \frac{\langle n_-^{PS} | \nabla_{\mathbf{P}} H^{PS} | n_+^{PS} \rangle}{E_+^{PS} - E_-^{PS}}. \tag{11}$$

The TDSE in the phase-space representation is thus

$$\dot{c}_i^{PS} = \sum_j^2 \Big( -iV_{ij} - \dot{\mathrm{R}} \cdot (\tau_{ij} + \tilde{d}_{ij}) - \dot{\mathbf{P}} \cdot \tilde{e}_{ij} \Big) c_j^{PS} \tag{12}$$

where

$$\begin{aligned} V_{ij} &= U^\dagger H_{ij} U \\ &= \begin{bmatrix} \tilde{E}_1 \cos^2(\frac{\theta}{2}) + \tilde{E}_2 \sin^2(\frac{\theta}{2}) & \frac{\tilde{E}_2 - \tilde{E}_1}{2}(\sin\theta) \\ \frac{\tilde{E}_2 - \tilde{E}_1}{2}(\sin\theta) & \tilde{E}_1 \sin^2(\frac{\theta}{2}) + \tilde{E}_2 \cos^2(\frac{\theta}{2}) \end{bmatrix} \end{aligned}$$

and

$$\begin{aligned} \tau_{ij} &= U^\dagger d_{ij} U \\ &= \mathbf{d}_{12} \dot{\mathbf{R}} \begin{bmatrix} -i\sin(\theta) & -i\cos(\theta) \\ -i\cos(\theta) & i\sin(\theta) \end{bmatrix}. \end{aligned}$$

According to the FSSH methodology, hops from adiabatic states $|\phi_i\rangle$ to $|\phi_j\rangle$ occur when the ratio of population being transferred from $|\phi_i\rangle$ to $|\phi_j\rangle$ exceeds a stochastically chosen parameter between 0 and 1.[3] In the SH literature the rate of population transfer from $|\phi_i\rangle$ to $|\phi_j\rangle$ is usually denoted by $b_{ji}$ and the net amount of population being transferred is $b_{ji} \cdot \Delta t$ where $\Delta t$ is the time-step. If $\zeta$ denotes the stochastic parameter, a hop is therefore invoked when the following condition is satisfied

$$\frac{b_{ji} \cdot \Delta t}{c_i^\dagger c_i} > \zeta. \tag{13}$$

Assuming the electronic wavefunction in FSSH is propagated in the adiabatic representation, $b_{ji}$ is calculated as follows, where $a_{ji} = c_j c_i^\dagger$

$$b_{ji} = -2\Re(a_{ji}^\dagger \cdot \mathbf{d}_{ji} \cdot \dot{\mathbf{R}}). \tag{14}$$

The same approach is used in PSSH. However the expression for $b_{ji}^{PS}$ (i.e. the rate of population transfer from $|n_i^{PS}\rangle$ to $|n_j^{PS}\rangle$) differs from that of FSSH. From Eq. (12), it is clear that there are four off-diagonal terms emerging from $V_{ij}$, $\tau_{ij}$, $\tilde{d}_{ij}$ and $\tilde{e}_{ij}$. These terms are required to calculate $b_{ji}^{PS}$

$$\begin{aligned} b_{ji}^{PS} &= 2\Im(a_{ji}^{PS\dagger} \cdot V_{ji}) - 2(\Re(a_{ji}^{PS\dagger} \cdot \tau_{ji} \cdot \dot{\mathbf{R}}) \quad (15) \\ &\quad + \Re(a_{ji}^{PS\dagger} \cdot \tilde{\mathbf{d}}_{ji} \cdot \dot{\mathbf{R}}) + \Re(a_{ji}^{PS\dagger} \cdot \tilde{\mathbf{e}}_{ji} \cdot \dot{\mathbf{P}}). \quad (16) \end{aligned}$$

The hopping rates in PSSH are not only proportional to nuclear velocities but also to changes in nuclear momentum due to the $\tilde{\mathbf{e}}_{ij} \cdot \dot{\mathbf{P}}$ term. An abrupt change in momentum can induce transitions between phase-space PES.[2]

## III. A COMMENT ON SUPERADIABATICITY

In Shenvi's original paper,[2] there was discussion of PSSH being a first-order superadiabatic correction to the adiabatic basis. However this is not strictly correct. A true first-order superadiabatic method[4,5] involves a change in basis that diagonalizes $H_{\mathit{eff}}$

$$H_{\mathit{eff}} = \sum_{j}^{2} \left( H_{ij} - i\dot{\mathbf{R}} \cdot \mathbf{d}_{ij} \right). \tag{17}$$

However the electronic basis used in PSSH does not diagonalize $H_{\mathit{eff}}$ but rather $H^{PS}$ (see Eq. (4)). The difference between them are their off-diagonal elements. In $H_{\mathit{eff}}$ those are $i\mathbf{d}_{ij} \cdot \dot{\mathbf{R}}$ and those in $H^{PS}$ are $i\mathbf{d}_{ij} \cdot \mathbf{P}/M$. Recall from the discussion in the main text that in PSSH, momentum and velocity are not simply variables related to one another through a mass-involving scaling factor and they can diverge in nonadiabatic regions. Hence the basis that diagonalizes $H^{PS}$ may not diagonalize $H_{\mathit{eff}}$ when $d_{ij}$ is significant.

[1] S. Hammes-Schiffer and J. C. Tully, J. Chem. Phys. **101**, 4657 (1994).
[2] N. Shenvi, J. Chem. Phys. **130**, 124117 (2009).
[3] J. C. Tully, J. Chem. Phys. **93**, 1061 (1990).
[4] M. V. Berry, Proc. R. Soc. London, Ser A **429**, 61 (1990).
[5] M. Deschamps, G. Kervern, D. Massiot, G. Pintacuda, L. Emsley, and P. J. Grandinetti, J. Chem. Phys. **129**, 204110 (2008).
